# Supplementary material for: Drifting mass accommodation coefficients: in situ measurements from a steady state molecular dynamics setup
Source: arXiv:2003.01022 ancillary file (2020-08-25)
Supplement: Supplementary file 1 [file Supplementary_Material.pdf]

Supplementary Material for

# Drifting mass accommodation coefficients: *in situ* measurements from a steady state molecular dynamics setup

Yigit Akkus[a], Akif Turker Gurer[a], Kishan Bellur[b,c]

[a]ASELSAN Inc., 06200 Yenimahalle, Ankara, Turkey
[b]Michigan Technological University, Houghton, MI 49931, USA
[c]University of Michigan, Ann Arbor, MI 48109, USA

A. Details of molecular dynamics simulations

B. Uncertainty analysis

## A. Details of molecular dynamics simulations

The numbers of fluid (Ar) and solid (Pt) atoms are 3783 and 4080, respectively. Walls are composed of 4 solid layers with (1,0,0) crystal planes facing the liquid. Lennard-Jones (L-J) 6-12 potential is used for the interactions between Ar-Ar and Ar-Pt. The interaction parameters utilized are: $\sigma_{Ar}$ = 0.34 nm, $\sigma_{Ar-Pt}$ = 0.3085 nm, and $\varepsilon_{Ar}$ = 0.01042 eV, $\varepsilon_{Ar-Pt}$ = 0.00558 eV [1]. Cut-off distance for the truncation of the L-J potential is selected as $3\sigma_{Ar}$. Embedded atom model is utilized to model Pt-Pt atomic interactions [2]. In order to eliminate the non-physical temperature jump caused by thermostats [3], heat transfer to/from fluid is performed by energy injection/extraction from selected solid atoms instead of thermostat application. Wall atoms located between heating and cooling zones are not allowed to vibrate to eliminate the undesirable heat conduction through the walls, otherwise the majority of energy is transferred *via* the solid medium, which is much more conductive than the fluid. Simulations are initiated from the Maxwell-Boltzmann velocity distribution for all atoms. A time step of 5 fs is used throughout the simulations. The simulation data (i.e. density, temperature, and velocity) are averaged for 5 ns. Simulations are carried out using Large-scale Atomic/Molecular Massively Parallel Simulator (LAMMPS) [4].

## B. Uncertainty analysis

Density, velocity (horizontal), and temperature are sampled at every 5 ns and all the data collected between the two measurements are averaged, which yields a measurement uncertainty, $\varepsilon$, for each time averaged data, $\langle .. \rangle$.

$$\rho = \langle \rho \rangle \pm \varepsilon_\rho \tag{S.1a}$$

$$u = \langle u \rangle \pm \varepsilon_u \tag{S.1b}$$

$$T = \langle T \rangle \pm \varepsilon_T \tag{S.1c}$$

Uncertainties associated with density ($\varepsilon_\rho$), velocity ($\varepsilon_u$), and temperature ($\varepsilon_T$) are estimated by calculating the standard error of measurements, which is evaluated by dividing the standard deviation of measurements to the number of samples.

Calculation of MAC coefficients is based on the respective kinetic theory equation (Hertz-Knudsen equation or a Schrage relation) and the measurement of the mass flow rate from the MD setup as summarized in Eqs. (2.4)-(2.6) of the manuscript. In order to demonstrate the uncertainty analysis, only one of these equations (Hertz-Knudsen: Eq.(2.4)) is considered here. If the measurement of the mass flux from MD setup is designated by $\dot{m}''$ and the mass flux prediction of Hertz-Knudsen equation (without multiplication with MAC) is designated by $\dot{m}''_{H-K}$, MAC coefficient can be expressed as follows:

$$\alpha^{H-K} = \left\langle \frac{\dot{m}''}{\dot{m}''_{H-K}} \right\rangle \pm \varepsilon_{\alpha^{H-K}} \tag{S.2}$$

Based on the concept of root of the sum of the squares uncertainty, the MAC coefficient's uncertainty ($\varepsilon_{\alpha^{H-K}}$) can be expressed as follows:

$$\varepsilon_{\alpha^{H-K}} = \sqrt{\left(\frac{\varepsilon_{\dot{m}''}}{\dot{m}''_{H-K}}\right)^2 + \left(\frac{\varepsilon_{\dot{m}''_{H-K}}\ \dot{m}''}{(\dot{m}''_{H-K})^2}\right)^2} \tag{S.3}$$

Uncertainty of the MAC coefficient ($\varepsilon_{\alpha^{H-K}}$) is simply due to the uncertainty associated with: (i) the measurement of the mass flux from MD setup ($\varepsilon_{\dot{m}''}$) and (ii) the calculation of mass flux from Hertz-Knudsen equation ($\varepsilon_{\dot{m}''_{H-K}}$). The next step is to determine these uncertainties.

Mass flux is simply the multiplication of density and velocity. Estimation of mass flux has associated uncertainty due to the time averaging of contributing terms:

$$\dot{m}'' = \langle \rho u \rangle \pm \varepsilon_{\dot{m}''} \tag{S.4}$$

Then uncertainty of the measured mass flux ($\varepsilon_{\dot{m}''}$) is expressed in terms of the uncertainties of density and velocity based on the concept of root of the sum of the squares uncertainty as follows:

$$\varepsilon_{\dot{m}''} = \sqrt{\left(\varepsilon_\rho u\right)^2 + (\varepsilon_u \rho)^2} \tag{S.5}$$

Calculation of mass flux from Hertz-Knudsen equation follows the relation below:

$$\dot{m}''_{H-K} = \left\langle \sqrt{\frac{k_b}{2\pi m}} \left(\rho^V \sqrt{T^V} - \rho_{sat}|_{T_i^L} \sqrt{T_i^L}\right) \right\rangle \pm \varepsilon_{\dot{m}''_{H-K}} \tag{S.6}$$

Then uncertainty of the calculated mass flux ($\varepsilon_{\dot{m}''_{H-K}}$) is expressed in terms of the uncertainties of densities and the temperatures based on the concept of root of the sum of the squares uncertainty as follows:

$$\varepsilon_{\dot{m}''_{H-K}} = \sqrt{\frac{k_b}{2\pi m}} \left[ \left(\varepsilon_{\rho^V} \frac{\partial \dot{m}''_{H-K}}{\partial \rho^V}\right)^2 + \left(\varepsilon_{T^V} \frac{\partial \dot{m}''_{H-K}}{\partial T^V}\right)^2 + \left(\varepsilon_{\rho_{sat}} \frac{\partial \dot{m}''_{H-K}}{\partial \rho_{sat}}\right)^2 + \left(\varepsilon_{T_i^L} \frac{\partial \dot{m}''_{H-K}}{\partial T_i^L}\right)^2 \right]^{0.5} \tag{S.7}$$

After carrying out differentiations and subsequent algebraic operations, uncertainty of the calculated mass flux becomes as follows:

$$\varepsilon_{\dot{m}''_{H-K}} = \sqrt{\frac{k_b}{2\pi m}}\left[\varepsilon_{\rho_v}^2 T_v + \frac{\varepsilon_{T_v}^2\ {\rho^V}^2}{4T^V} + \varepsilon_{\rho_{sat}}^2 T_i^L + \frac{\varepsilon_{T_i^L}^2\ \rho_{sat}^2}{4T_i^L}\right]^{0.5} \tag{S.8}$$

When Eq. S5 and Eq. S8 are inserted into Eq. S3, uncertainty of the MAC coefficient is obtained.

## References

[1] S. Maruyama and T. Kimura. A study on thermal resistance over a solid-liquid interface by the molecular dynamics method. *Therm. Sci. Eng.*, 7(1):63-68, 1999.

[2] S. M. Foiles, M. I. Baskes, and M. S. Daw. Embedded-atom-method functions for the fcc metals Cu, Ag, Au, Ni, Pd, Pt, and their alloys. *Phys. Rev. B*, 33(12):7983, 1986.

[3] M. Barisik and A. Beskok. Boundary treatment effects on molecular dynamics simulations of interface thermal resistance. *J. Comput. Phys.*, 231(23):7881-7892, 2012.

[4] S. Plimpton. Fast parallel algorithms for short-range molecular dynamics. *J. Comput. Phys.*, 117(1):1-19, 1995.
